# Supplementary material for: Robust Sparse Voting
Source: arXiv:2202.08656 source file (2024-01-25)
Supplement: Supplementary file 1 [file app-additional-rel-work.tex]

\section{Additional related work}
\label{sec:additional-rel-work}
